# Supplementary material for: Laser spectroscopy of neutron-rich $^{207,208}$Hg isotopes: Illuminating the kink and odd-even staggering in charge radii across the $N=126$ shell closure
Source: arXiv:2012.13802 source file (2020-12-26)
Supplement: Supplementary file 1 [file Hg-NR-SupMat.pdf]

# Laser spectroscopy of neutron-rich $^{207,208}$Hg isotopes: Illuminating the kink and odd-even staggering in charge radii across the $N = 126$ shell closure

T. Day Goodacre,[1,2,3,*] A.V. Afanasjev,[4] A.E. Barzakh,[5] B.A. Marsh,[2] S. Sels,[2,6] P. Ring,[7] H. Nakada,[8] A.N. Andreyev,[9,10] P. Van Duppen,[6] N.A. Althubiti,[1,11] B. Andel,[6,12] D. Atanasov,[13,†] J. Billowes,[1] K. Blaum,[13] T.E. Cocolios,[1,6] J.G. Cubiss,[9] G.J. Farooq-Smith,[1,6] D.V. Fedorov,[5] V.N. Fedosseev,[2] K.T. Flanagan,[1,14] L.P. Gaffney,[6,15,‡] L. Ghys,[6,16] M. Huyse,[6] S. Kreim,[13,2] D. Lunney,[17,§] K.M. Lynch,[1,2] V. Manea,[13,§] Y. Martinez Palenzuela,[6,2] P.L. Molkanov,[5] M. Rosenbusch,[18,19] R.E. Rossel,[2,20] S. Rothe,[2] L. Schweikhard,[18] M.D. Seliverstov,[5] P. Spagnoletti,[15] C. Van Beveren,[6] M. Veinhard,[2] E. Verstraelen,[6] A. Welker,[2,21] K. Wendt,[20] F. Wienholtz,[2,18,¶] R.N. Wolf,[13,18,**] A. Zadvornaya,[6] and K. Zuber[21]

[1] *The University of Manchester, School of Physics and Astronomy, Oxford Road, M13 9PL Manchester, United Kingdom*
[2] *CERN, CH-1211 Geneva 23, Switzerland*
[3] *TRIUMF, Vancouver V6T 2A3, Canada*
[4] *Department of Physics and Astronomy, Mississippi State University, MS 39762, USA*
[5] *Petersburg Nuclear Physics Institute, NRC Kurchatov Institute, Gatchina 188300, Russia*
[6] *KU Leuven, Instituut voor Kern- en Stralingsfysica, B-3001 Leuven, Belgium*
[7] *Fakultät für Physik, Technische Universität München, D-85748 Garching, Germany*
[8] *Department of Physics, Graduate School of Science, Chiba University, Yayoi-cho, I-33, Inage, Chiba 263-8522, Japan*
[9] *Department of Physics, University of York, York, YO10 5DD, United Kingdom*
[10] *Advanced Science Research Center (ASRC), Japan Atomic Energy Agency (JAEA), Tokai-mura, Japan*
[11] *Physics Department, Faculty of Science, Jouf University, Aljouf, Saudi Arabia*
[12] *Department of Nuclear Physics and Biophysics, Comenius University in Bratislava, 84248 Bratislava, Slovakia*
[13] *Max-Planck-Institut für Kernphysik, Saupfercheckweg 1, 69117 Heidelberg, Germany*
[14] *The Photon Science Institute, The University of Manchester, Manchester, M13 9PL, United Kingdom*
[15] *School of Computing, Engineering, and Physical Sciences, University of the West of Scotland, Paisley PA1 2BE, United Kingdom*
[16] *Belgian Nuclear Research Center SCK•CEN, Boeretang 200, B-2400 Mol, Belgium*
[17] *CSNSM-IN2P3, Université de Paris Sud, Orsay, France*
[18] *Universität Greifswald, Institut für Physik, 17487 Greifswald, Germany*
[19] *RIKEN Nishina Center, Wako, Japan*
[20] *Institut für Physik, Johannes Gutenberg-Universität, D-55099 Mainz, Germany*
[21] *Institut für Kern- und Teilchenphysik, Technische Universität Dresden, Dresden 01069, Germany*

## OVERVIEW

This supplemental material includes the method of extracting the change in the nuclear mean square charge radius from the measured isotope shifts. Table I lists the numerical kink parameter ($\Delta R^{(3)}(A)$) values that are presented graphically in Fig. 4 (a) and (b). Table II lists the absolute charge radius values from RHB(DD-ME2) and NR-HFB(M3Y-P6a) calculations for lead and mercury isotopes at $N$=126.

## EXTRACTION OF $\delta\langle r^2\rangle^{A,A'}$

The change in the mean square charge radius of the isotope with mass number $A$, relative to the isotope with mass number $A'$, $\delta\langle r^2\rangle^{A,A'}$, was extracted from $\delta\nu^{A,A'}$ via standard methods [1] using the relation

$$\delta\nu^{A,A'} = F_\lambda K(Z)\delta\langle r^2\rangle^{A,A'} + M \times \frac{A - A'}{A'A}, \tag{1}$$

where for the 253.65-nm transition the electronic factor is $F_{254} = -55.36(39)$ GHz fm$^{-2}$ [2, 3], $K(Z)$ is a correction factor which accounts for higher-order radial moments $K(Z = 80) = 0.931$ (taking into account [2] and [4]), and $M$ is the mass shift factor (the sum of the normal mass shift, $M_{\text{NMS}}$, and the specific mass shift, $M_{\text{SMS}}$, factors) $M = (1 \pm 0.5) \cdot M_{\text{NMS}}$ [3]. The same atomic factors were used in [5, 6].

## $\Delta R^{(3)}(A)$ VALUES

The kink indicator, $\Delta R^{(3)}(A)$, values calculated using Eq. (2) of the main text are presented in Table I. These values are presented graphically in Figs. 4 (a) and 4 (b) of the main text together with additional information on the theoretical approaches.

| $Z$ | Expt. (fm) | M3Y-P6a (fm) | DD-ME2 (fm) | DD-ME2_np (fm) | Fy(Δr) (fm) | UNEDF1 (fm) |
|---|---|---|---|---|---|---|
| 80 | 0.0048(3) | 0.0027 | 0.0052 | | | 0.0002 |
| 82 | 0.0042(3) | 0.0025 | 0.0044 | 0.0051 | 0.0078 | 0.0002 |

TABLE I: Experimental (mercury: this work; lead: calculated from Ref. [7]) and theoretical (M3Y-P6a, DD-ME2, DD-ME2-np: this work; Fy(Δr): Ref. [8]; UNEDF1: Ref. [9]) $\Delta R^{(3)}(A)$ values, considering $A = 208$ and $A = 206$ for lead and mercury, respectively. Reference $R$ values were taken from Ref. [10].

## $R$ VALUES

Table II presents absolute charge radius values at $N$=126 from RHB(DD-ME2) and NR-HFB(M3Y-P6a) calculations, together with literature data.

| $Z$ | Expt. (fm) | M3Y-P6a (fm) | DD-ME2 (fm) |
|---|---|---|---|
| 80 | 5.484(4) | 5.428 | 5.499 |
| 82 | 5.501(1) | 5.446 | 5.518 |

TABLE II: Experimental $R$ values are taken from Ref. [10] and theoretical (DD-ME2 and M3Y-P6a) values from this work.

* tdaygoodacre@triumf.ca
† Present address: CERN, 1211, Geneva 23, Switzerland.
‡ Present address: Department of Physics, University of Liverpool, Liverpool, L69 7ZE, United Kingdom
§ Present address: Université Paris-Saclay, CNRS/IN2P3, IJCLab, 91405 Orsay, France.
¶ Present address: Institut für Kernphysik, Technische Universität Darmstadt, 64289 Darmstadt, Germany.
** Present address: ARC Centre of Excellence for Engineered Quantum Systems, School of Physics, The University of Sydney, NSW 2006, Australia.

[1] E. W. Otten, Nuclear Radii and Moments of Unstable Isotopes, in *Treatise on Heavy Ion Science* (Springer US, Boston, MA, 1989) pp. 517–638.
[2] G. Torbohm, B. Fricke, and A. Rosén, State-dependent volume isotope shifts of low-lying states of group-II a and -II b elements, Phys. Rev. A **31**, 2038 (1985).
[3] G. Ulm *et al.*, Isotope shift of $^{182}$Hg and an update of nuclear moments and charge radii in the isotope range $^{181}$Hg-$^{206}$Hg, Z. Phys. A: Hadrons Nucl. **325**, 247 (1986).
[4] G. Fricke and K. Heilig, *Nuclear Charge Radii*, 1st ed., edited by H. Schopper, Landolt-Börnstein - Group I Elementary Particles, Nuclei and Atoms, Vol. 20 (Springer-Verlag, Berlin/Heidelberg, 2004) pp. 1–419.
[5] B. A. Marsh *et al.*, Characterization of the shape-staggering effect in mercury nuclei, Nat. Phys. **14**, 1163 (2018).
[6] S. Sels *et al.*, Shape staggering of mid-shell mercury isotopes from in-source laser spectroscopy compared with Density Functional Theory and Monte Carlo Shell Model calculations, Phys. Rev. C **99**, 044306 (2019).
[7] M. Anselment, W. Faubel, S. Göring, A. Hanser, G. Meisel, H. Rebel, and G. Schatz, The odd-even staggering of the nuclear charge radii of Pb isotopes, Nucl. Phys. A **451**, 471 (1986).
[8] C. Gorges *et al.*, Laser Spectroscopy of Neutron-Rich Tin Isotopes: A Discontinuity in Charge Radii across the N=82 Shell Closure, Phys. Rev. Lett. **122**, 192502 (2019).
[9] Mass Explorer, http://massexplorer.frib.msu.edu. Accessed:2020-06-01.
[10] I. Angeli and K. Marinova, Table of experimental nuclear ground state charge radii: An update, At. Data Nucl. Data Tables **99**, 69 (2013).
